# Supplementary material for: Charged Lepton Flavour Violation in Heavy Particle DEcays
Source: arXiv:2205.10576 source file (2022-05-21)
Supplement: Supplementary file 1 [file supplemental.tex]

\subsection{Doubly-charged Scalar}

The doubly-charged scalar $H^{\pm\pm}$ exists in a large variety of BSM scenarios, such as the type-II seesaw~\cite{Magg:1980ut, Schechter:1980gr, Cheng:1980qt, Lazarides:1980nt, Mohapatra:1980yp}, LRSM~\cite{Pati:1974yy, Mohapatra:1974gc, Senjanovic:1975rk} and the Zee-Babu model~\cite{Babu:1988ki}. The doubly-charged scalars can couple either to left-handed or right-handed charged fermions in the SM, and the most general Yukawa couplings can be written in the form of
\begin{eqnarray}
{\cal L}_Y = f_{\alpha\beta} H^{++} \overline{\ell_\alpha^C} \ell_\beta ~+~ {\rm H.c.} \,,
\end{eqnarray}
which is not only LNV but also potentially LFV. The most stringent limit on the doubly-charged scalar mass $M_{\pm\pm}$ is from the direct searches of same-sign dilepton pairs from $H^{\pm\pm}$ decay at the LHC~\cite{ATLAS:2017xqs, CMS:2017pet}. At the low-energy high-precision frontier, the coupling $f_{\alpha\beta}$ is also constrained by the LFV decays $\ell_\alpha \to \ell_\beta \gamma$, $\ell_\alpha \to \ell_\beta \ell_\gamma \ell_\delta$, the electron and muon $g-2$, muonium-antimuonium oscillation and the LEP $e^+ e^- \to \ell^+ \ell^-$ data (see e.g. Ref.~\cite{BhupalDev:2018vpr}).

The doubly-charged scalar can be pair produced at the high-energy lepton and hadron colliders via its gauge interactions, i.e. $e^+ e^-,\, pp \to H^{++} H^{--}$. However, the gauge interaction induced Drell-Yan processes can not be used to directly probe the Yukawa couplings $f_{\alpha\beta}$, unless the Yukawa couplings are sufficiently small such that $H^{\pm\pm}$ is long-lived at the colliders. As for the neutral scalar $H$ case above, the doubly-charged scalar $H^{\pm\pm}$ can also be singly produced at the high-energy lepton colliders via the Yukawa couplings $f_{\alpha\beta}$~\cite{Rizzo:1981dla, Lusignoli:1989tr, Barenboim:1996pt, Kuze:2002vb, Yue:2007kv, Yue:2007ym}. 
%e.g. $e^+ e^- \to H^{\pm\pm} \ell_\alpha^\mp \ell_\beta^\mp$. 
%The corresponding production cross section of this channel is proportional to  the Yukawa coupling $|f_{\alpha\beta}|^2$, therefore the Yukawa coupling $f_{\alpha\beta}$ can be directly measured in such processes. 
Take $f_{e\mu}$ as an explicit example, with the $e^\pm$ beams and the the high-energy photon beams, we can have the following single production processes
\begin{eqnarray}
e^+ e^- ,\, \gamma\gamma \to H^{\pm\pm} e^\mp \mu^\mp  \,, \quad
e^\pm \gamma \to H^{\pm\pm} \mu^\mp \,.
%\gamma\gamma \to H^{\pm\pm} e^\mp \mu^\mp \,.
\end{eqnarray}
For simplicity, we assume the doubly-charged scalar decays predominately into $e^\pm \mu^\pm$. The prospects of $H^{\pm\pm}$ at the ILC 1 TeV with luminosity of 1 ab$^{-1}$ are shown in Fig.~\ref{fig:Hpp}. For the photon beam, we take the effective photon luminosity distribution from Refs.~\cite{Ginzburg:1981vm, Ginzburg:1982yr, Telnov:1989sd}. In the $e^+ e^-$ and $\gamma\gamma$ channels, for doubly-charged scalar mass $M_{\pm\pm} \lesssim \sqrt{s}=500$ GeV, the production of $H^{\pm\pm}$ will be dominated by the Drell-Yan process, while for $M_{\pm\pm}\gtrsim 500$ GeV only the single production of $H^{\pm\pm}$ is kinematically allowed. The $e^\pm \gamma$ process has only two particles in the final state, thus it can probe a smaller Yukawa coupling $f_{e\mu}$. The shaded regions in Fig.~\ref{fig:Hpp} are excluded by the LEP $ee \to \mu\mu$ data and the direct searches at the LHC~\cite{CMS:2017pet,ATLAS:2017iqw}. The contribution of doubly-charged scalars to the muon $g-2$ is always negative, and therefore can not explain the muon $g-2$ anomaly. Furthermore,  the doubly-charged scalar contribution to muon $g-2$ is highly suppressed by the charged lepton mass~\cite{Lindner:2016bgg}, thus not shown in Fig.~\ref{fig:Hpp}. As illustrated in Fig.~\ref{fig:Hpp}, the coupling $f_{e\mu}$ of the doubly-charged scalar $H^{\pm\pm}$ can be directly measured at the future high-energy lepton colliders via searches of the LFV signals, even if the current stringent LFV constraints are taken into consideration.

%which can be ensured if the coupling $f_{e\mu}$ is much larger than other Yukawa couplings and other decay channels of the doubly-charged scalar such as $H^{\pm\pm} \to W^\pm W^\pm$ are subdominant. 
%With ${\rm BR} (H^{\pm\pm} \to e^\pm \mu^\pm)=100\%$, the corresponding LHC limit on $M_{\pm\pm}$ is shown as the vertical dashed line in Fig.~\ref{fig:Hpp}~\cite{ATLAS:2017iqw,CMS:2017pet}. The coupling $f_{e\mu}$ will also induce extra contribution to $e^+ e^- \to \mu^+ \mu^-$ at the LEP, and the corresponding limit is presented as the pink shaded region in Fig.~\ref{fig:Hpp:1}. 

\begin{figure}[t!]
  \centering
  \includegraphics[width=0.6\textwidth]{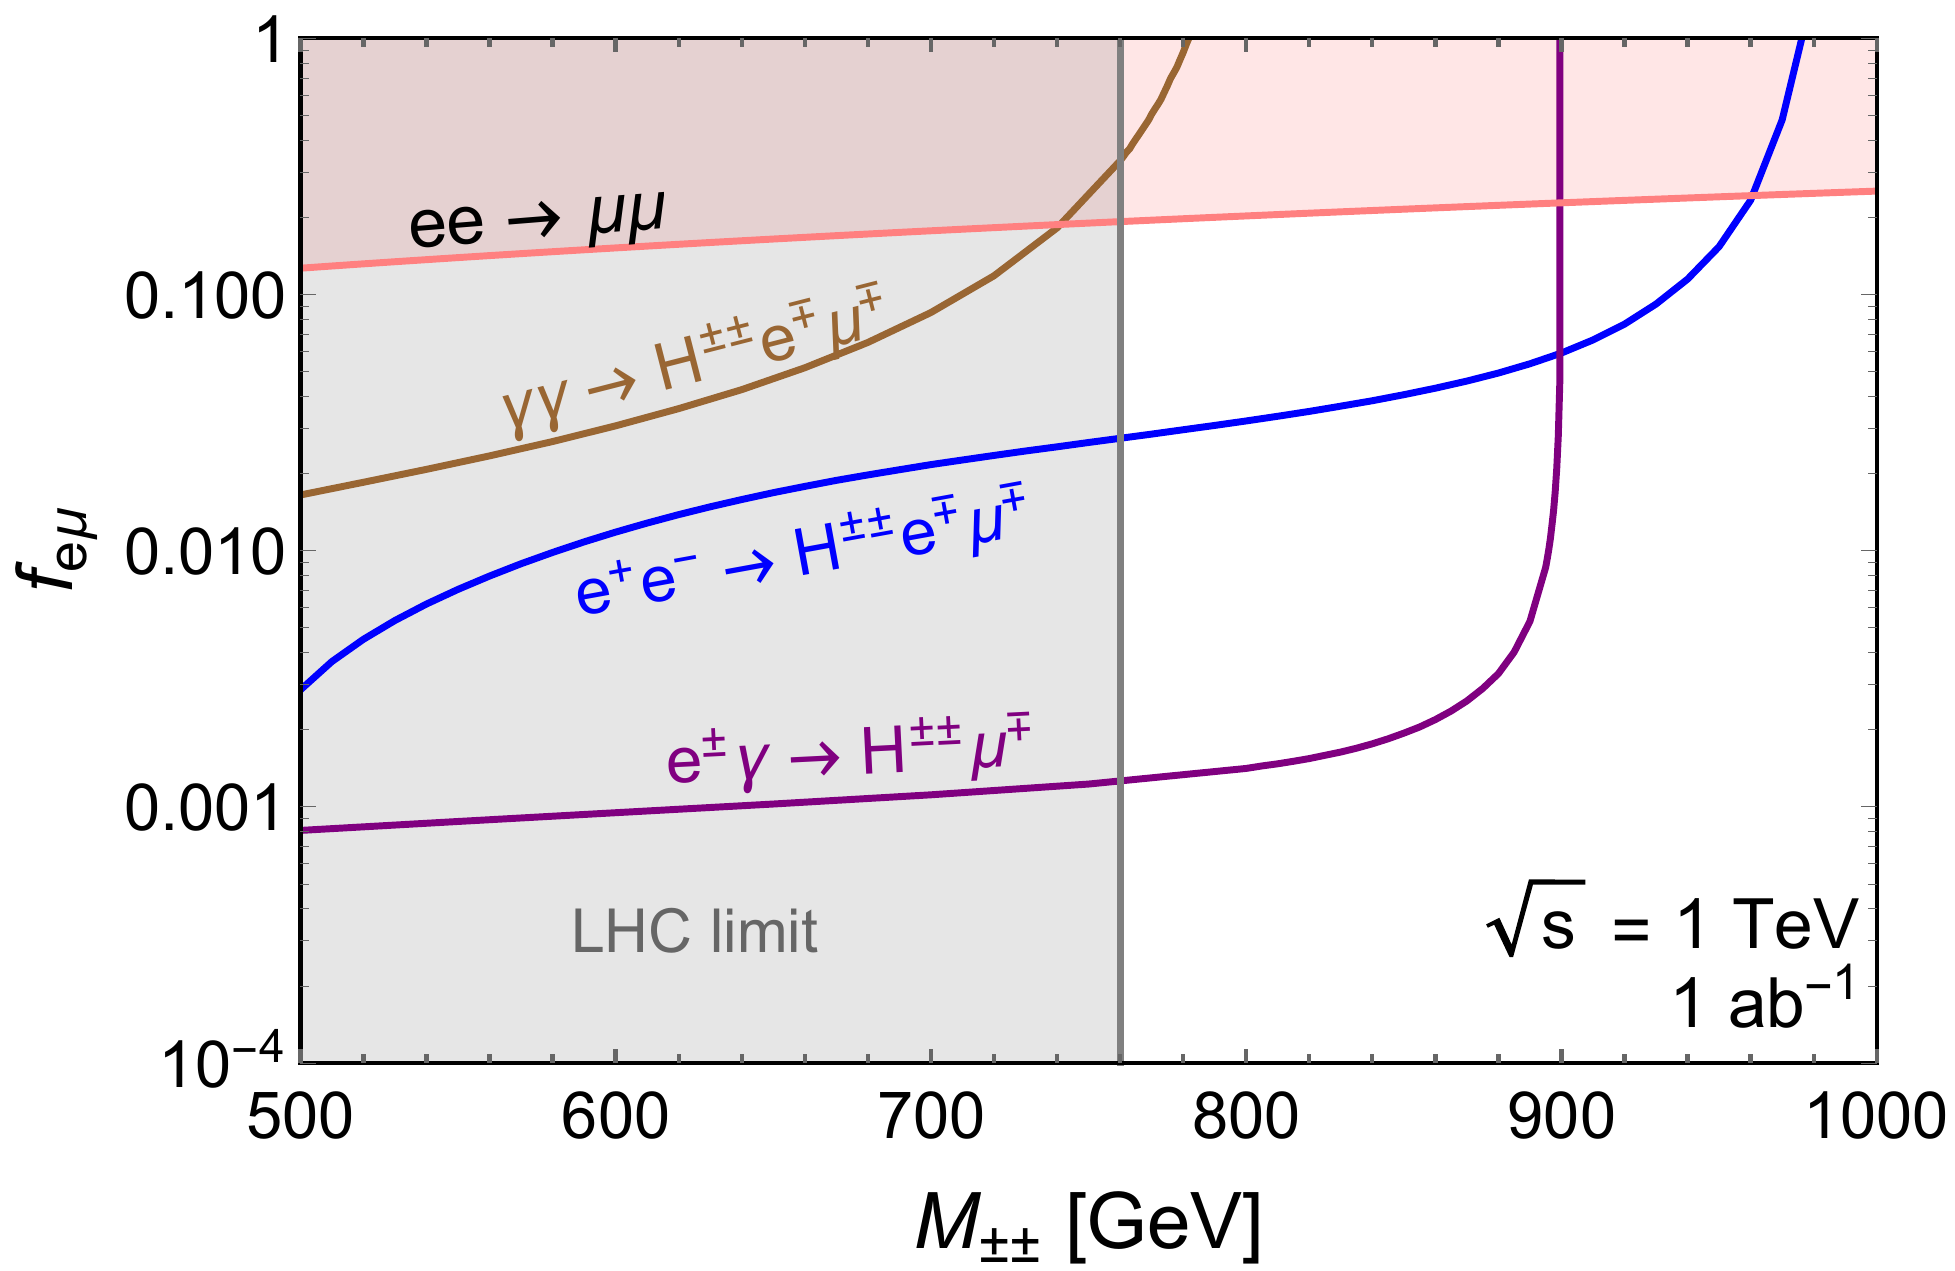} 
  \caption{Prospects of the doubly-charged scalar mass $M_{\pm\pm}$ and the LFV coupling $f_{e\mu}$ at ILC $1$ TeV with 1 ab$^{-1}$, in the $e^+ e^-$ (blue), $e\gamma$ (purple) and $\gamma\gamma$ (brown) production processes. The gray pink shaded regions are excluded respectively by the LHC limit assuming ${\rm BR} (H^{\pm\pm} \to e^{\pm} \mu^{\pm}) = 100\%$ and the LEP $ee \to \mu^+ \mu^-$ data. Figure from Ref.~\cite{BhupalDev:2018vpr}.}
  \label{fig:Hpp}
\end{figure}

For the LFV coupling $f_{e\tau}$, the prospects at the ILC 1 TeV is to some extent similar to the $f_{e\mu}$ case, with a smaller reconstruction efficiency for $\tau$ than muons. For the LFV coupling $f_{\mu\tau}$, the production cross section for $e^+ e^-,\, \gamma\gamma \to H^{\pm\pm}\mu^\mp \tau^\mp$ is much smaller than that for $H^{\pm\pm} e^\mp \mu^\mp$ and $H^{\pm\pm} e^\mp \tau^\mp$. As a result, the prospects of $f_{\mu\tau}$ are only at the order of 0.1~\cite{BhupalDev:2018vpr}.

\begin{figure}[t!]
  \centering
  \includegraphics[width=0.45\textwidth]{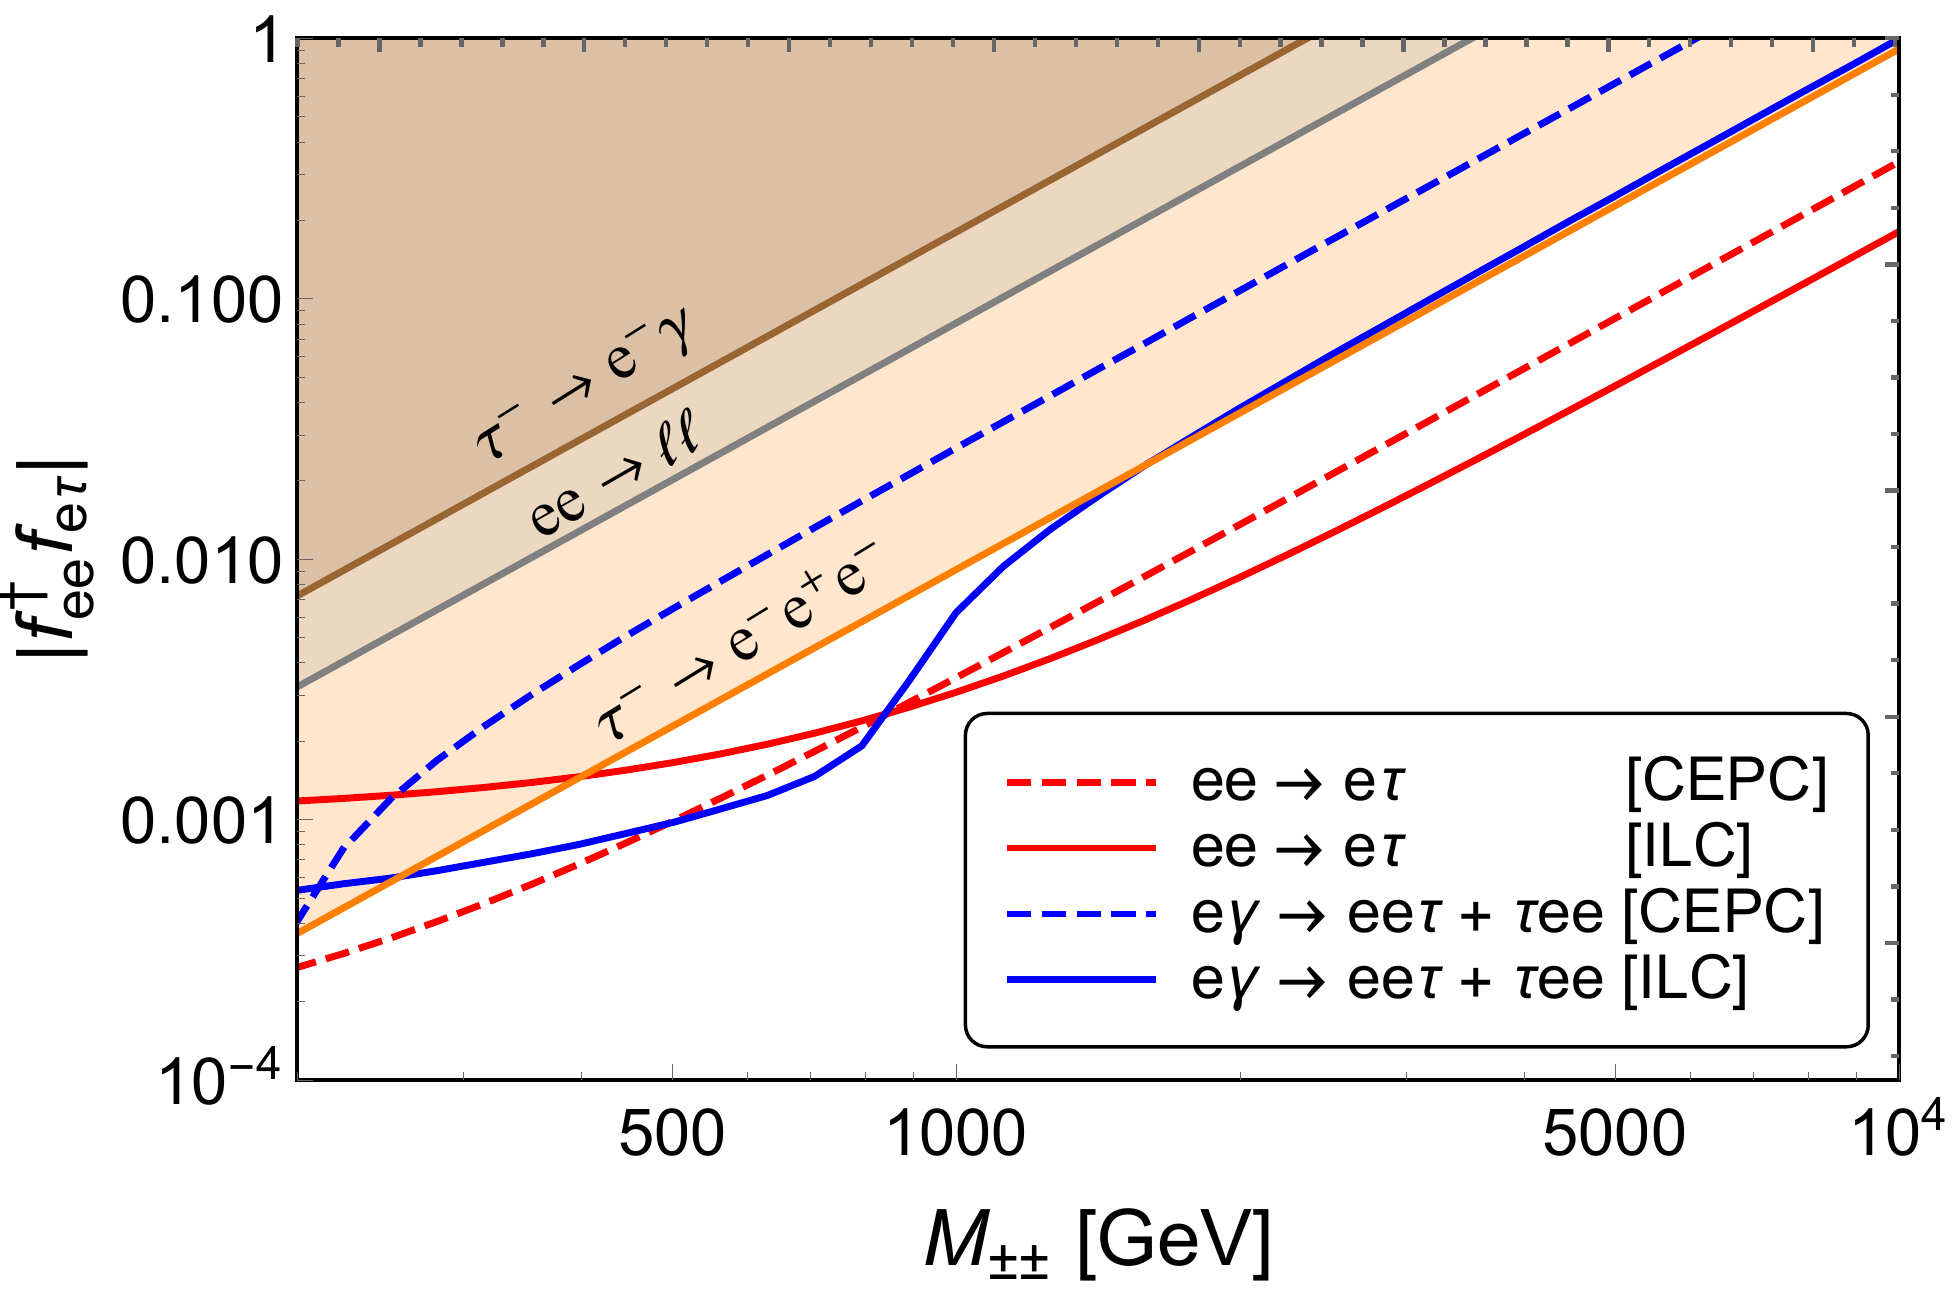}
  \includegraphics[width=0.45\textwidth]{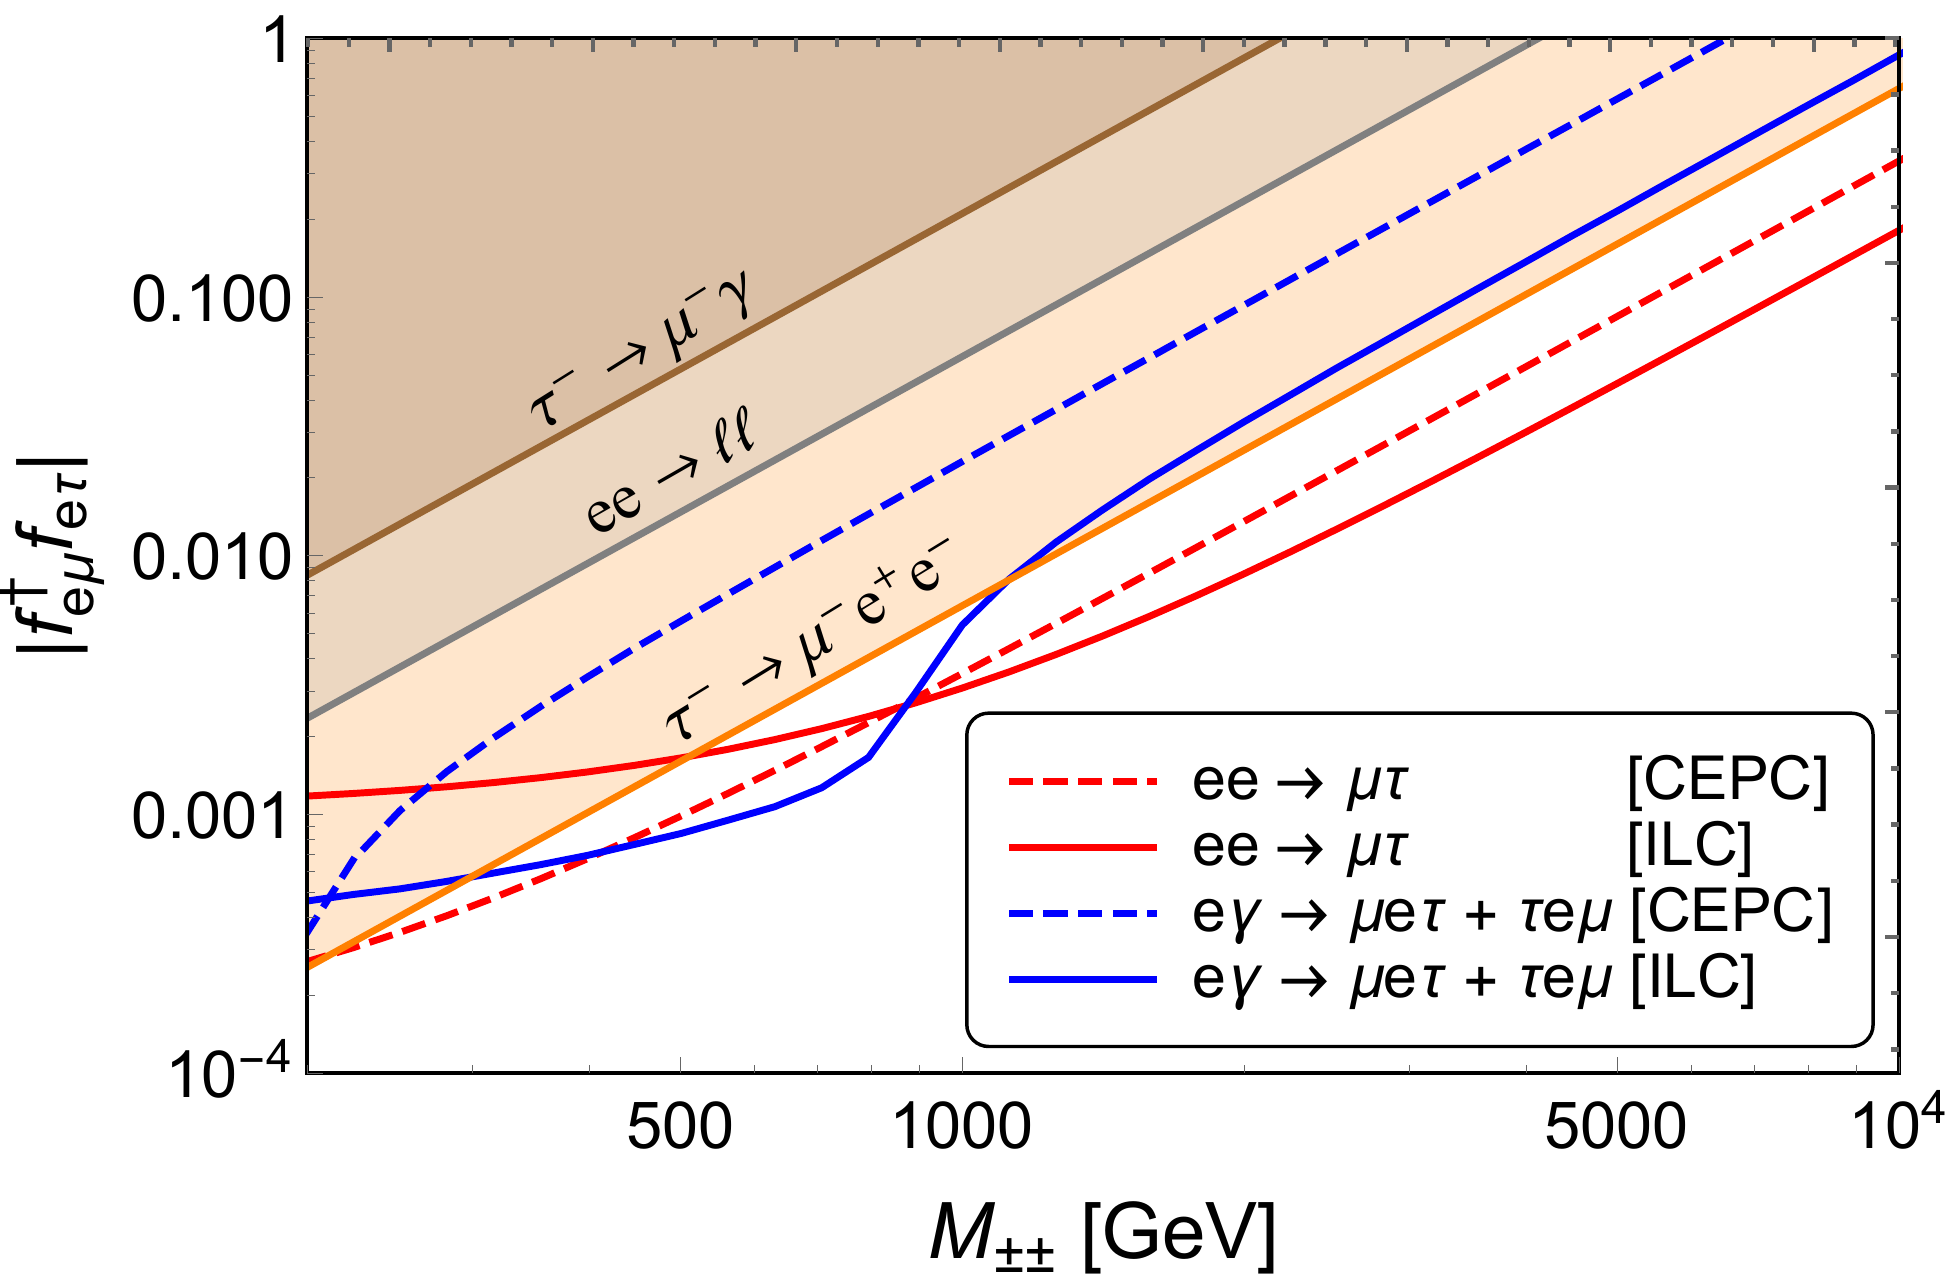}
  \caption{Prospects of the Yukawa couplings $|f_{ee}^\dagger f_{e\tau}|$ (left) and $|f_{e\mu}^\dagger f_{e\tau}|$ (right) for the doubly-charged scalar $H^{\pm\pm}$ production via the $ee \to \ell_\alpha \ell_\beta$ (red) and $e\gamma \to \ell_\alpha \ell_\beta \ell_\gamma$ (blue) processes, at CEPC with 240 GeV with 5 ab$^{-1}$ (dashed) and ILC 1 TeV with 1 ab$^{-1}$ (solid). The shaded regions are excluded by the corresponding limits. Figure from Ref.~\cite{BhupalDev:2018vpr}.}
  \label{fig:Hpp:2}
\end{figure}

As in the case of neutral scalar $H$ above, as a mediator the doubly-charged scalar $H^{\pm\pm}$ can induce the LFV processes
\begin{eqnarray}
\label{eqn:dcs:offshell}
e^+ e^- \to \ell_\alpha^\pm \ell_\beta^\mp \,, \quad
e^\pm \gamma \to \ell_\alpha^\pm \ell_\beta^\pm \ell_\gamma^\mp \,.
\end{eqnarray}
The limit from $\mu \to eee$ is so stringent that it precludes the prospects of $H^{\pm\pm}$ in the channel of $e^\pm \mu^\mp$. In the $\tau$ flavor sector, the coupling $f_{ee}^\dagger f_{e\tau}$ and $f_{e\mu}^\dagger f_{e\tau}$ will induce respectively the processes $e^+ e^- \to e^\pm \tau^\mp$, $e^\pm \gamma \to e^\pm e^\pm \tau^\mp$, $\tau^\pm e^\pm e^\mp$ and $e^+ e^- \to \mu^\pm \tau^\mp$, $e^\pm \gamma \to \mu^\pm e^\pm \tau^\mp$, $\tau^\pm e^\pm \mu^\mp$. The corresponding prospects at the high-energy lepton colliders are shown respectively in the left and right panels of Fig.~\ref{fig:Hpp:2}. The red and blue lines are respectively for the $e^+ e^-$ and $e^\pm\gamma$ channels, and the dashed and solid lines are respectively for the sensitivities at CEPC 240 GeV and ILC 1 TeV. The relevant limits from rare LFV tau decay and the LEP data are labelled by the shaded regions. As in the neutral scalar case in Section~\ref{sec:theory:Hdecay}, both CEPC and ILC can probe $H^{\pm\pm}$ with mass larger than the center-of-mass energy in the $e^+ e^-$ channel, which corresponds to detecting the effective four-fermion interaction $(\overline{e}e)(\overline{\ell}_\alpha\ell_\beta)$ with the cut-off scale $\Lambda \simeq M_{\pm\pm}/\sqrt{|f_{}^\dagger f_{}|}$. More $H^{\pm\pm}$ induced LFV processes such as $e\gamma \to \mu\mu\mu,\, \mu\mu\tau$ are also possible, but the corresponding prospects are suppressed by the small cross sections. More details can be found in Ref.~\cite{BhupalDev:2018vpr}.

%With three particles in the final state, the cross section for $e\gamma$ processes are not as competitive as the $e^+ e^-$ channel, as seen in the left panel of Fig.~\ref{fig:Hpp:2}. 

%Similar to the neutral scalar case, the relevant limits for the doubly-charged scalar are from the LFV decays $\tau \to e \gamma$, $\tau \to eee$ and the LEP data $\ell^+ \ell^-$ data, which are presented as the shaded regions in the left panel of Fig.~\ref{fig:Hpp:2}. 

%The dashed lines denote the CEPC sensitivities, and  the solid lines are for ILC. 

%Given the coupling $f_{e\mu}^\dagger f_{e\tau}$, the doubly-charged scalar $H^{\pm\pm}$ can induce the processes $e^+ e^- \to \mu^\pm \tau^\mp$ and $e^\pm \gamma \to \mu^\pm e^\pm \tau^\mp,\, \tau^\pm e^\pm \mu^\mp$, and the corresponding limits from $\tau^- \to \mu^-\gamma$, $\tau^-\to \mu^- e^+ e^-$, the LEP $\ell^+ \ell^-$ data and prospects at the CEPC 240 GeV and ILC 1 TeV are presented in the right panel of Fig.~\ref{fig:Hpp:2}. As for the case of $f_{ee}^\dagger f_{e\tau}$, the $e^+ e^-$ processes have better sensitivities than the $e\gamma$ collisions. These processes can also be induced by the coupling $f_{ee}^\dagger f_{\mu\tau}$, However, the corresponding production cross sections are smaller, which weakens the detectability of $f_{ee}^\dagger f_{\mu\tau}$ at future high-energy lepton colliders. 

\subsection{Heavy Neutrinos}

In the type-I seesaw~\cite{Minkowski:1977sc,Mohapatra:1979ia, Yanagida:1979as,Gell-Mann:1979vob,Glashow:1979nm}, heavy Majorana neutrinos are introduced to generate the tiny neutrino masses. In some other seesaw models such as the inverse seesaw~\cite{Mohapatra:1986aw, Mohapatra:1986bd, Bernabeu:1987gr}, the heavy neutrinos can also be (pseudo-)Dirac fermions, or even mixture of Dirac and Majorana states. In general, 
%No matter being either Majorana or Dirac fermions, 
the heavy neutrinos $N$ mix with the active neutrinos $\nu_\alpha$, and thus couple to the SM $W$ and $Z$ bosons through the heavy-light neutrino mixing $V_{\alpha N}$. If the heavy neutrinos are at or below the TeV-scale, they can be produced at the high-energy lepton and hadron colliders. 
%For simplicity, let us focus here only on the LFV signals from the heavy neutrinos. To this end, let us neglect the specific UV completions of seesaw models and consider only one heavy neutrino $N = N_1$, with the other two states $N_{2,3}$ much heavier and not contributing significantly to the LFV signals. 
For instance, the heavy neutrino $N$ can be produced at $pp$ colliders via the charged current Drell-Yan and vector-boson fusion (VBF) process~\cite{Datta:1993nm, Dev:2013wba, Alva:2014gxa, Degrande:2016aje} 
\begin{eqnarray}
\label{eqn:N}
&&q\bar{q}^\prime \to W^{\pm\ast} \to \ell_\alpha^\pm N \to \ell_\alpha^\pm \ell_\beta^{\mp,\,\pm} W^{\pm,\,\mp} \,, \nonumber \\
&& W^{\pm\ast} \gamma \to \ell_\alpha^\pm N \to \ell_\alpha^\pm \ell_\beta^{\mp,\,\pm} W^{\pm,\,\mp} \,,
\end{eqnarray}
where we have assumed the heavy neutrino mass $m_N > m_W$ (with $m_W$ the $W$ boson mass). If the heavy neutrino $N$ is a Dirac fermion, there will only be opposite-sign charged leptons $\ell_\alpha^\pm \ell_\beta^\mp$ in the final state. For the case of Majorana $N$, there will also be the same-sign charged leptons $\ell_\alpha^\pm \ell_\beta^\pm$, which is  undoubtedly LNV signals beyond the SM. 
%As a result of the Majorana nature in the type-I seesaw, the heavy neutrinos will generate same-sign lepton signatures at the high-energy colliders, which is
%For some mass ranges of $m_N$, the gluon-fusion process $gg\to Z^\ast,\, h^\ast \to \nu N$ is also very important~\cite{Willenbrock:1985tj,Dicus:1991wj, Hessler:2014ssa}.  More details about the production channels of $N$ can be found e.g. in Ref.~\cite{Pascoli:2018heg}. 
If the heavy neutrino $N$ mixes with two neutrino flavors $\nu_{\alpha,\,\beta}$ (with $\alpha\neq \beta$) in the SM, the production and decay of $N$ at the high-energy colliders will produce LFV signals, i.e. $\ell_\alpha\neq\ell_\beta$ in the final state of the process in Eq.~(\ref{eqn:N}) via the charged currents.

\begin{figure}[t!]
  \centering
  \includegraphics[width=0.55\textwidth]{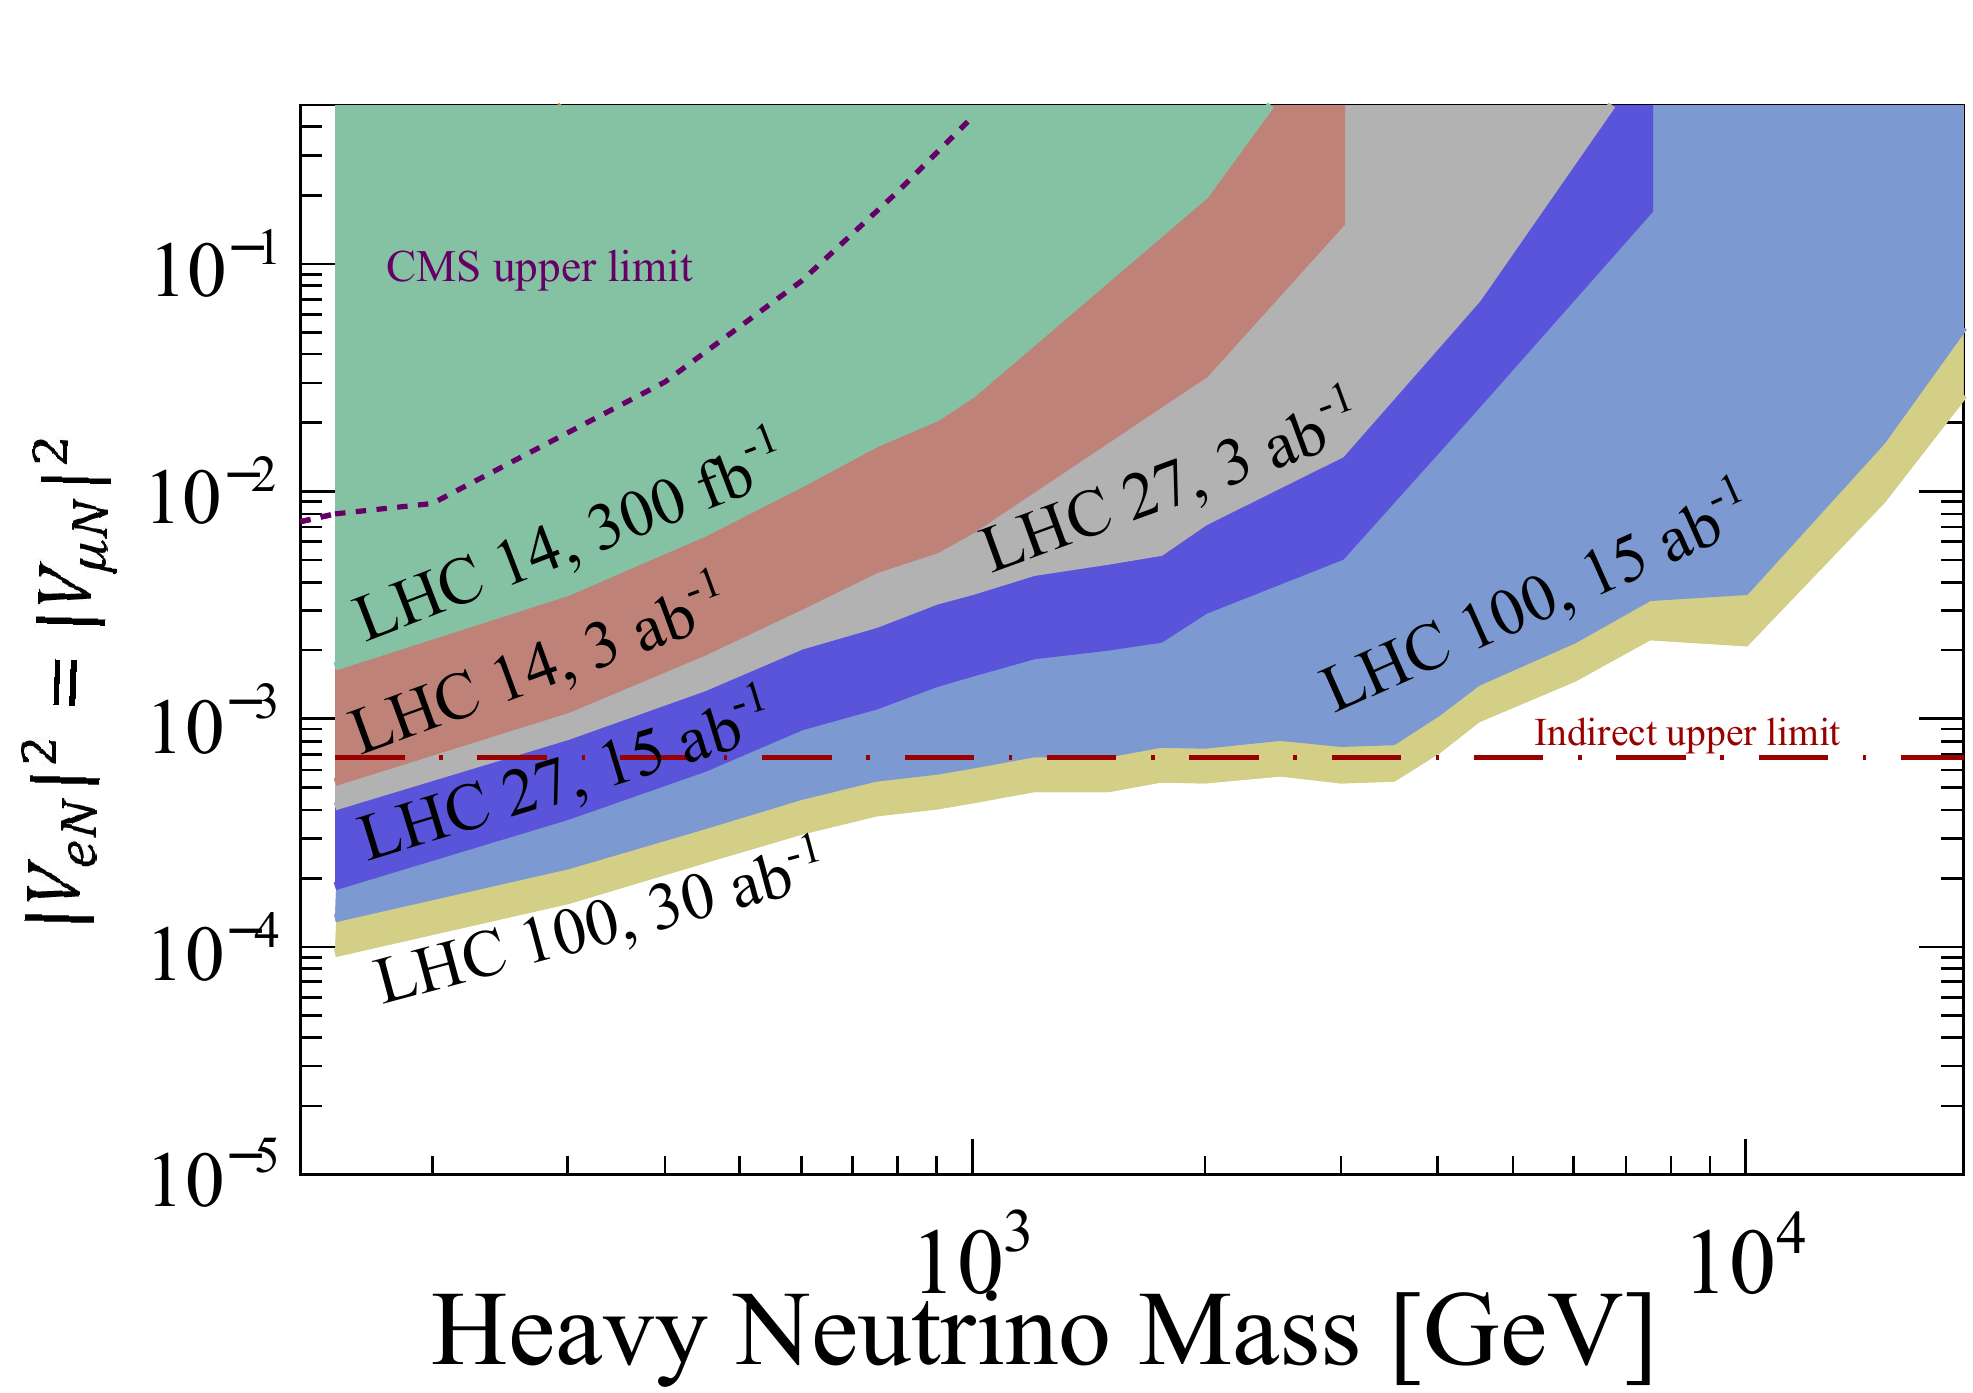} 
  \caption{Sensitivities of heavy neutrino mass $m_N$ and the heavy-light neutrino mixing $|V_{eN}|^2 = |V_{\mu N}|^2$, at future LHC 14 TeV with luminosities of 300 fb$^{-1}$ and 3 ab$^{-1}$, LHC 27 TeV with 3 ab$^{-1}$ and 15 ab$^{-1}$, and 100 TeV collider with 15 ab$^{-1}$ and 30 ab$^{-1}$. Regions above the short dashed line are excluded by the CMS data, and the dot-dashed horizontal line indicates the indirect limit from current EWPD data. Figure from Ref.~\cite{Pascoli:2018heg}.}
  \label{fig:N}
\end{figure}

If the $W$ boson in the final state of Eq.~(\ref{eqn:N}) decays leptonically, we will have three charged leptons plus significant missing transverse energy (MET) in the final state, with potentially extra (VBF) jets. With $|V_{eN}| = |V_{\mu N}|$, we can have the processes $pp \to ee\ell_X + e\mu\tau_h$, with $\tau_h$ referring to the hadronic decaying tauons, $\ell_X = e,\, \mu,\,\tau_h$, and all the possible lepton charges are included. 
%Adopting dynamic jet vetoes, 
The resultant sensitivities of $m_N$ and the heavy-light neutrino mixing $|V_{eN}| = |V_{\mu N}|$ at future hadron colliders are presented in Fig.~\ref{fig:N}~\cite{Pascoli:2018heg}. The prospects here are not sensitive to the Majorana or Dirac nature of $N$. In the near future, the LHC 14 TeV data with a luminosity of 300 fb$^{-1}$ can probe a mixing $|V_{eN}|^2 = |V_{\mu N}|^2 \sim {\cal O} (10^{-3})$ for a heavy neutrino at the scale of 100 GeV. At future 100 TeV collider, the sensitivity of heavy-light neutrino mixing can even go down to ${\cal O}(10^{-4})$. 
%To obtain these results, the simulations of $N$ production is implemented with {\tt MadGraph5}~\cite{Alwall:2014hca} and parton showering and hadronization by using {\tt Pythia8}~\cite{Sjostrand:2014zea}. Next-to-leading order (NLO) corrections in QCD are taken into consideration, and  the hadron particles are clustered by using {\tt FastJet}~\cite{Cacciari:2011ma} with the anti-$k_T$ algorithm~\cite{Cacciari:2008gp}. 
More simulation details can be found in Ref.~\cite{Pascoli:2018heg}. In Fig.~\ref{fig:N}, the regions above the short dashed line are excluded by the direct trilepton searches of $N$ at CMS~\cite{CMS:2018iaf}, and horizontal dot-dashed line represents the current electroweak precision data (EWPD) constraints on $|V_{\alpha N}|$~\cite{Fernandez-Martinez:2016lgt}. 
%More limits on the heavy-light neutrino mixing can be found e.g. in Ref.~\cite{Bolton:2019pcu}.

%\textcolor{blue}{[YZ: working on the following paragraphs...]}

When $N$ is relatively light, say at the GeV-scale, it can be directly produced in meson decays~\cite{Atre:2009rg,Coloma:2020lgy}. In the charged meson sector, the heavy neutrino will induce the decay 
\begin{eqnarray}
\label{eqn:meson}
{\cal P}_2^\pm \to \ell_\alpha N^{(\ast)} \to \ell_\alpha^\pm \ell_\beta^{\mp,\,\pm} {\cal P}_1^{\pm,\,\mp} \,, 
%\ell_\alpha^\pm \ell_\beta^{\pm} {\cal P}_1^\mp \,,
\end{eqnarray}
with ${\cal P}_{1,\,2}^\pm$ the charged mesons. This process will be LFV if $N$ mixes with two flavors of active neutrinos $\nu_{\alpha,\,\beta}$, which results in $\ell_\alpha\neq \ell_\beta$ via the charged-current interactions. The LNV decays $\ell_\alpha^\pm \ell_\beta^{\pm} {\cal P}_1^\mp$ are also possible if $N$ is a Majorana fermion. It is found that in the mass range of $m_\pi < m_N < m_K$ (with $m_{\pi,\,K}$ the masses of pions and Kaons), the most stringent limit on $|V_{eN}V_{\mu N}|$ is from the decay $K^+ \to \pi^+ e^\pm \mu^\mp$ leading to $|V_{eN}V_{\mu N}|\lesssim 10^{-9}$~\cite{Hu:2019zan}. For $m_K < m_N < m_B$ (with $m_{B}$ the $B$ meson mass), the strongest limit is from $B^+ \to \pi^+ e^\pm \mu^\mp$~\cite{Hu:2019zan}. In the process (\ref{eqn:meson}), if $N$ is on-shell, it can be directly searched via the two-body meson decays, e.g. $K^+ \to \ell^+ N$. The NA62 data have excluded $|V_{eN}|^2 ,\, |V_{\mu N}|^2 \lesssim 10^{-8}$ to $10^{-9}$ for $170\, {\rm MeV} < m_N < 450$ MeV~\cite{NA62:2017qcd}. More relevant processes can be found e.g. in Refs.~\cite{Coloma:2020lgy,Bolton:2019pcu}. For neutral mesons such as ${\cal P}^0=K_L$, $D^0$, $B^0$, $B_s^0$, the heavy neutrino can induce LFV leptonic decays at the 1-loop level, i.e.
\begin{eqnarray}
{\cal P}^0 \to \ell_\alpha^\pm \ell_\beta^\mp \,.
\end{eqnarray}
%which can be applied to the LFV leptonic decays of $K_L$, $D^0$, $B^0$, and $B_s^0$. 
Such LFV meson decays are all highly suppressed in the SM, and the mass $m_N$ and heavy-light neutrino mixing $|V_{\alpha N} V_{\beta N}|$ are tightly constrained by precision meson data. 
%When $N$ is heavier than the $B$ mesons, the best limit is from $B_s^0 \to e^\pm \mu^\mp$. 
More details can be found e.g. in Ref.~\cite{Hu:2019zan}. 

In the charged lepton sector, if $N$ mixes with two flavors of active neutrinos, it will contribute to the radiative LFV decays of charged leptons $\ell_\alpha \to \ell_\beta\gamma$ and $\mu - e$ conversion in nuclei. It is found that the most stringent limit is from $\mu \to e \gamma$, which leads to $|V_{eN} V_{\mu N}| \lesssim 10^{-3}$ for a 10 GeV $N$~\cite{Bolton:2019pcu}.

%Before leaving this section, we would like to comment that 
%If two (or more) heavy neutrino $N_{1,\,2}$ are involved, there could be more phenomenological implications, such as heavy neutrino mixing and CP violation due to the TeV-scale $N$~\cite{Bray:2007ru} or in the decays of mesons and the SM Higgs~\cite{Tapia:2021gne, Cvetic:2021lmm, Abada:2019bac}. All these processes might involve LFV in some way.

\subsection{Heavy $W_R$ Boson}

The $W_R$ boson in the LRSM mediate right-handed charged-currents, and couples directly to the heavy neutrinos $N$. The primary direct search channel of $W_R$ boson at the high-energy hadron colliders is via
\begin{eqnarray}
q\bar{q}^\prime \to W_R^{\pm} \to \ell_\alpha^\pm N \to \ell_\alpha^\pm \ell_\beta^{\pm} W_R^{\mp\ast} \to 
\ell_\alpha^\pm \ell_\beta^\pm jj \,, 
\end{eqnarray}
where we have assumed  the heavy neutrinos are lighter than the $W_R$ bosons, and the same-sign dilepton in the final state is from the Majorana nature of the heavy neutrino $N$. In such a process, the heavy neutrino mass eigenstate $N$ may be a state of pure flavor $\alpha$, or combinations of two flavors $\alpha$ and $\beta$, i.e. $N = \cos\theta N_\alpha + \sin\theta N_\beta$ with $\theta$ the mixing angle of heavy neutrinos $N_{\alpha,\,\beta}$. The latter case will lead to LFV signatures $\ell_\alpha^\pm \ell_\beta^\pm$ via the $W_R$-mediated charged-currents. The current most stringent LHC limit has excluded $W_R$ mass up to 5.4 TeV based on the data of 138 fb$^{-1}$ at 13 TeV, covering the lepton flavor combinations $\ell_\alpha^\pm \ell_\beta^\pm = e^\pm e^\pm, \, \mu^\pm \mu^\pm,\, e^\pm \mu^\pm$~\cite{CMS:2021dzb}. 

With 3000 fb$^{-1}$ data at 14 TeV, the $W_R$ mass can be probed up to roughly 6.5 TeV~\cite{Nemevsek:2018bbt, Chauhan:2018uuy}. At future 100 TeV colliders, the $W_R$ mass prospect can be further improved up to roughly 40 TeV with a luminosity of 10 fb$^{-1}$, assuming the heavy neutrino decays promptly~\cite{Mitra:2016kov, Ruiz:2017nip}. If the neutrino $N$ is light, the parameter space of $W_R$-mediated three-body decay $N \to \ell jj$ will be highly compressed. This will make $N$ long-lived at the high-energy colliders, with the decay length of $N$ up to the meter level for $m_N \sim 10$ GeV~\cite{Nemevsek:2018bbt, Helo:2013esa}. The displaced vertex signals from $N$ decay can be used to search for the heavy $W_R$ boson, and the  prospect of $W_R$ mass can go up to 33 TeV at the future 100 TeV collider, with $m_N \sim 100$ GeV~\cite{Nemevsek:2018bbt}. The prompt and displaced vertex signals from $W_R$ and $N$ can both be sources for LFV signatures at the future high-energy hadron colliders.
